# Supplementary material for: Counterfactual Story Reasoning and Generation
Source: arXiv:1909.04076 source file (2019-09-12)
Supplement: Supplementary file 1 [file supplementary.tex]

%
% File emnlp2019.tex
%
%% Based on the style files for ACL 2019, which were
%% Based on the style files for EMNLP 2018, which were
%% Based on the style files for ACL 2018, which were
%% Based on the style files for ACL-2015, with some improvements
%%  taken from the NAACL-2016 style
%% Based on the style files for ACL-2014, which were, in turn,
%% based on ACL-2013, ACL-2012, ACL-2011, ACL-2010, ACL-IJCNLP-2009,
%% EACL-2009, IJCNLP-2008...
%% Based on the style files for EACL 2006 by 
%%e.agirre@ehu.es or Sergi.Balari@uab.es
%% and that of ACL 08 by Joakim Nivre and Noah Smith

\documentclass[11pt,a4paper]{article}
\usepackage[hyperref]{emnlp-ijcnlp-2019}
\usepackage{times}
\usepackage{latexsym}
\usepackage{bm}
\usepackage{amsmath}
\usepackage{amssymb}
\usepackage{multirow}
\usepackage{xspace}
\usepackage{graphicx}
\usepackage{color}
\usepackage{makecell}
\usepackage{booktabs}
\usepackage{array}
\usepackage{booktabs}
\usepackage{color,colortbl}
\usepackage{tabularx}
\usepackage{soul}

\usepackage{url}

%\aclfinalcopy % Uncomment this line for the final submission

%\setlength\titlebox{5cm}
% You can expand the titlebox if you need extra space
% to show all the authors. Please do not make the titlebox
% smaller than 5cm (the original size); we will check this
% in the camera-ready version and ask you to change it back.

\title{
%Counterfactual Reasoning:\\ Story Rewriting with Minimum Edit
Counterfactual Story Reasoning and Generation Supplementary Materials
}

\author{First Author \\
  Affiliation / Address line 1 \\
  Affiliation / Address line 2 \\
  Affiliation / Address line 3 \\
  {\tt email@domain} \\\And
  Second Author \\
  Affiliation / Address line 1 \\
  Affiliation / Address line 2 \\
  Affiliation / Address line 3 \\
  {\tt email@domain} \\}

\date{}

\begin{document}
\maketitle

\appendix

\input{supp-appendix.tex}

\bibliography{emnlp-ijcnlp-2019}
\bibliographystyle{acl_natbib}

\end{document}
